# Supplementary material for: Variational Variance: Simple, Reliable, Calibrated Heteroscedastic Noise Variance Parameterization
Source: arXiv:2006.04910 source file (2020-10-30)
Supplement: Supplementary file 1 [file supplement.tex]

% text commands
\newcommand{\blankSection}{This section is intentionally blank since its supplemental section is not necessary.}
\newcommand{\captionVAE}[1]{VAE PPC Visualization for #1: The rows within a subplot from top to bottom are randomly selected test data followed by the posterior predictive mean and variance and a sample from it. Pixel values are clamped to $[0,1]$, when PPC values exit this interval.}

\section{Introduction}
Hereafter, we include supplementary material for our manuscript. Please refer to our \href{https://arxiv.org/abs/2006.04910}{arxiv} version for the latest results. Our code is available at \url{https://github.com/astirn/VariationalVariance}. We organize this supplement using the same section names as the main article. Any reference to the supplement from the main article will appear in the corresponding section. Figure and table numbers continue from the main article.

\section{Amortized Variational Inference}
\blankSection

\section{Variational Variance for Regression}

\subsection{Existing Methods We Use as Baselines}
\blankSection

\subsection{Proposed Regression Methods}
The following derivation proves that precision's true posterior for regression locally factorizes into a distribution that depends both on the covariates $x_i$ and responses $y_i$. As we discuss in the main article, this dual dependence implies the true posterior falls outside the scope of heteroscedasticity due to the additional dependence on $y_i$.
\begin{align*}
	p(\lambda | y, x) 
		&= \frac{p(y,\lambda|x)}{p(y|x)}
			= \frac{p(y,\lambda|x)}{\int p(y,\lambda|x) d\lambda}
			= \frac{p(y|x,\lambda)p(\lambda)}{\int p(y,\lambda|x) d\lambda}\\
		&= \frac{\prod_{i=1}^n \N(y_i|\mu(x_i), \lambda_i) p(\lambda_i)}
                {\int \prod_{i=1}^n \N(y_i|\mu(x_i), \lambda_i) p(\lambda_i)d\lambda_i}\\
		&= \frac{\prod_{i=1}^n \N(y_i|\mu(x_i), \lambda_i) p(\lambda_i)}
                {\prod_{i=1}^n \int \N(y_i|\mu(x_i), \lambda_i) p(\lambda_i)d\lambda_i}\\
		&= \prod_{i=1}^n p(\lambda_i|y_i,x_i)
\end{align*}
Above, we use $p(\lambda_i|y_i,x_i) \triangleq \frac{\N(y_i|\mu(x_i), \lambda_i) p(\lambda_i)}{\int \N(y_i|\mu(x_i), \lambda_i) p(\lambda_i)d\lambda_i}$ to symbolically capture the local factorization.

\subsubsection{Precision Priors}
Here, we derive the xVAMP ELBO and decompose its KL divergence. The xVAMP generative process is
\begin{align*}
	u_1,\hdots,u_K &\sim \text{UniformWithoutReplacement}(\{x_1,\hdots,x_N\})\\
	\lambda_i|x_i &\sim p(\lambda_i|x_i,u_1,\hdots,u_K) \triangleq \sum_{j=1}^K \pi_j(x_i) \cdot q(\lambda_i|u_j)\\
	y_i|x_i,\lambda_i &\sim p(y_i|x_i,\lambda_i) \triangleq \mathcal{N}(y_i|\mu(x_i),\lambda_i).
\end{align*}
Please note that we treat $\{u_j\}_{j=1}^K$ as prior parameters (not random variables).

\clearpage
This generative process leads to the local (per-point) ELBO
\begin{align*}
	\log p(y_i|x_i)
		&= \E_{q(\lambda_i|x_i)} \Bigg[\log p(y_i|x_i,\lambda_i) - \log\frac{q(\lambda_i|x_i)}{p(\lambda_i|x_i)} + \log\frac{q(\lambda_i|x_i)}{p(\lambda_i|x_i,y_i)} \Bigg]\\
		&= \E_{q(\lambda_i|x_i)} \big[\log p(y_i|x_i,\lambda_i)\big] - D_{KL}\big(q(\lambda_i|x_i)||p(\lambda_i|x_i)\big) + D_{KL}\big(q(\lambda_i|x_i)||p(\lambda_i|x_i,y_i)\big)\\
		&\geq \E_{q(\lambda_i|x_i)} \big[\log p(y_i|x_i,\lambda_i)\big] - D_{KL}\big(q(\lambda_i|x_i)||p(\lambda_i|x_i)\big)\\
		&= \E_{q(\lambda_i|x_i)} \Bigg[\log p(y_i|x_i,\lambda_i) - \log q(\lambda_i|x_i) + \log \sum_{j=1}^K \pi_j(x_i) q(\lambda_i|u_j)\Bigg].
\end{align*}
From the ELBO, we determine
\begin{align}
	D_{KL}\big(q(\lambda_i|x_i)||p(\lambda_i|x_i)\big)
		&= \E_{q(\lambda_i|x_i)} \Bigg[\log q(\lambda_i|x_i) - \log \sum_{j=1}^K \pi_j(x_i) q(\lambda_i|u_j)\Bigg]\nonumber\\
		&= -\mathbb{H}\big[q(\lambda_i|x_i)\big] - \E_{q(\lambda_i|x_i)}\Bigg[\log \sum_{j=1}^K \pi_j(x_i) q(\lambda_i|u_j)\Bigg]\label{eq:dkl}.
\end{align}

For VBEM's prior parameters we use the Cartesian square of a set of scalars ranging from 0.05 to 4.0. That set of integers is
$$\{0.05, 0.1, 0.25, 0.5, 0.75, 1.0, 1.5, 2.0, 2.5, 3.0, 3.5, 4.0\}.$$

\begin{figure}[b!]
    \centering
    \includegraphics[width=0.99\textwidth]{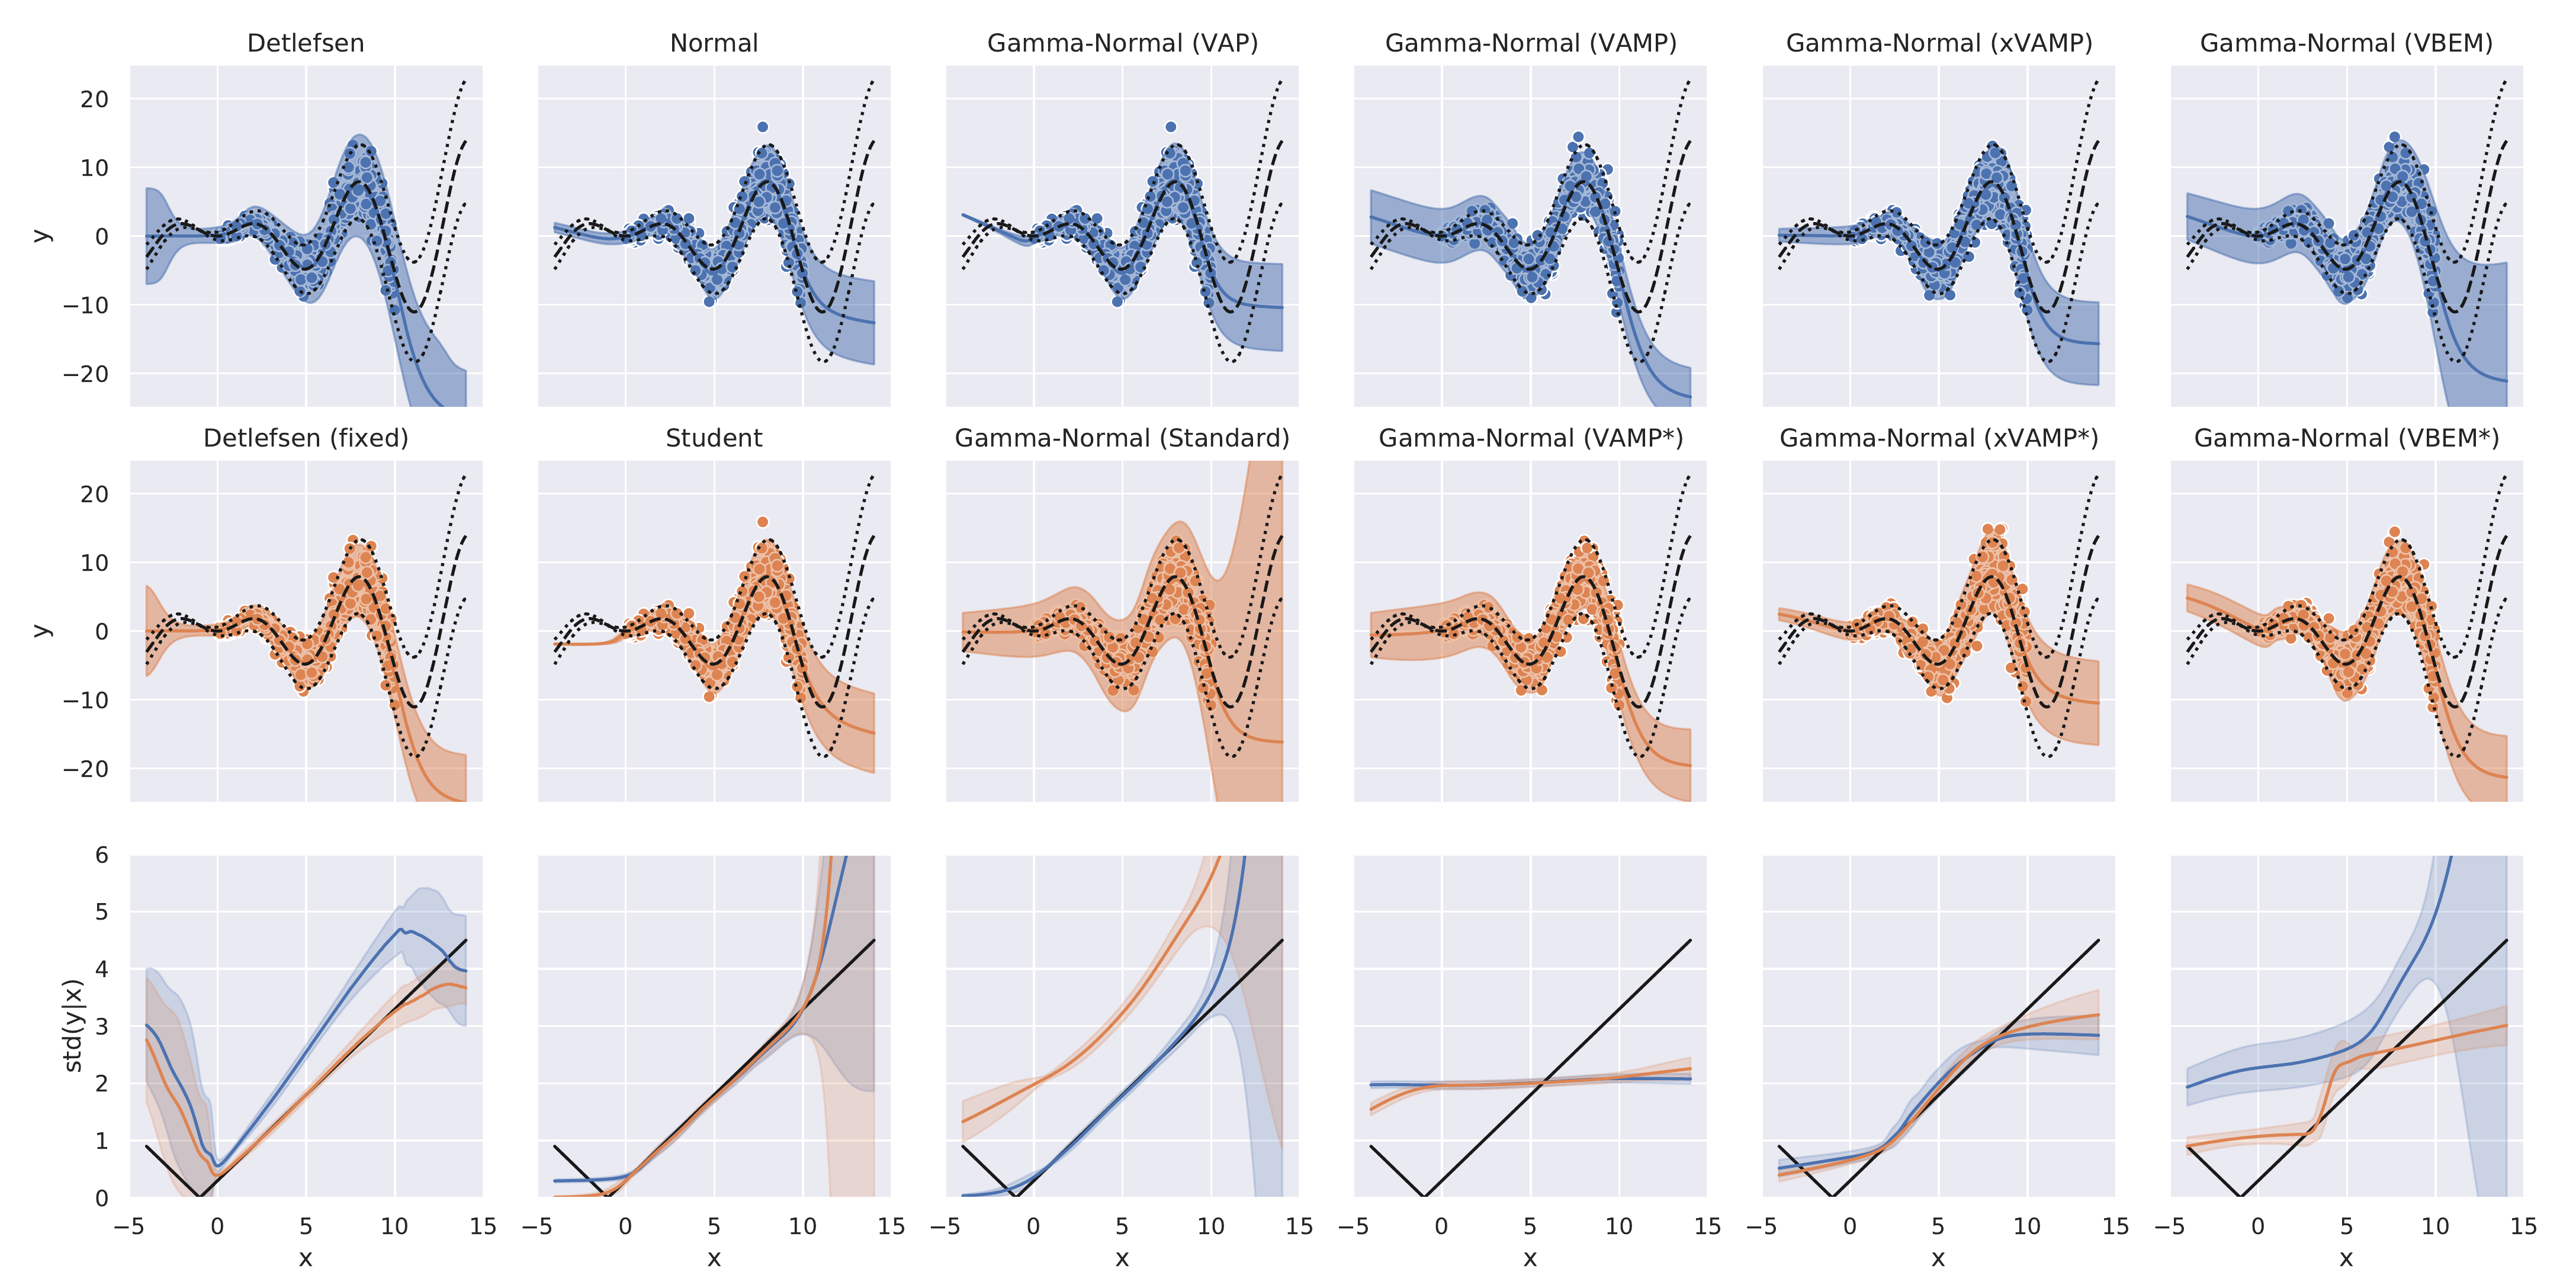}
    \caption{Toy Regression Results. Top two rows: dots are training data, black dashed/dotted lines and colored lines/areas are the true and predictive $\E[x|y] \pm 2 \cdot \sqrt{\var(y|x)}$, respectively. Third row: the true (black) and average predictive (colors correspond to methods above) $\sqrt{\var(y|x)}$ for 20 trials (area is one deviation).}
    \label{fig:toy-big}
\end{figure}

\subsection{Toy Data}
Here, we provide the exact implementation details used during the toy regression experiments. For all methods, we employ neural networks with a single hidden layer of 50 sigmoid neurons to match \cite{detlefsen2019reliable}. For our VAMP($^*$), xVAMP($^*$), and VBEM$^*$ priors, we set $K=20$. For VAMP($^*$) and xVAMP($^*$), we sample pseudo-inputs $u_i\iid\Uni([-4,14])$. Like \cite{detlefsen2019reliable}, we use ADAM \citep{kingma2014adam} for optimization. While \cite{detlefsen2019reliable} employ separate optimizers for the mean and variance networks that respectively use 1e-2 and 1e-3 as learning rates, we employ a single ADAM instance with a learning rate of 5e-3. We run all algorithms for 6e3 epochs without batching (i.e. the single batch contains all 500 training points). We ran the toy experiments on a NVIDA RTX2070.

We additionally include an enlarged copy (\cref{fig:toy-big}) of the main article's toy data figure for enhanced clarity.

\subsection{UCI Data}
Here, we provide the experimental specifics for the UCI regression experiments. \cite{detlefsen2019reliable} again employ a neural network with a single hidden layer, but now with 50 ReLU neurons.  We use the same network architecture except with ELU neurons, which we found to be more robust during our Monte-Carlo estimation of the right-most term of \cref{eq:dkl}'s RHS. The baseline code \citep{detlefsen2019reliable} allows training to run for some number of batch iterations, whereas our code uses the notion of an epoch, which encompasses the number of batches required to see each example in the training set exactly once. To keep things equal, we allow each algorithm to run for a dataset-specific number of batch iterations with a batch size of 256, which we convert to epochs ($\lceil\frac{\text{iterations}}{\text{batch size}}\rceil$) for our methods.  All UCI datasets use 2e4 batch iterations except for those with larger ($N > 9000$) sample sizes (e.g. carbon, naval, power plant, and superconductivity), which use 1e5 batch iterations. Here, \cite{detlefsen2019reliable} use 1e-2 and 1e-4 as learning rates for the mean and variance networks, respectively. We use 1e-3 as the learning rate for our single ADAM instance. We use $a=1$ and $b=0.001$ as the standard Gamma prior's parameters. For VAMP($^*$) and xVAMP($^*$) we sample $K=100$ pseudo-inputs uniformly from the training set without replacement. We also use $K=100$ for our VBEM$^*$ prior. We employ early stopping on the validation set's log (posterior) predictive likelihood with a patience of 50 epochs. We implemented an equivalent early stopping mechanism in the baseline code \citep{detlefsen2019reliable}, in which we also introduced support for multivariate response variables. We ran the UCI experiments on a NVIDA RTX2070 and were able to parallelize up to five trials (i.e. five concurrent training sessions for any of the tested models).

We include the remaining PPC metrics in \cref{tab:uci-mean-bias,tab:uci-mean-RMSE,tab:uci-var-bias,tab:uci-var-RMSE,tab:uci-samp-bias,tab:uci-samp-RMSE}, where we bold just the top performer. We italicize any cited (i.e. reported) results, which we never bold since we did not validate those methods under our experimental configurations (e.g. some reported results use larger neural networks). Statistical ties for all PPC metrics are tallied in table 2 of our original manuscript.

\begin{table}[ht!]
    \caption{UCI Mean Bias \meanpmstd \ \tuple}
    \label{tab:uci-mean-bias}
    \begin{center}
	    {\scriptsize \begin{tabular}{lllllll}
\toprule
             &       &                   boston &                        carbon &                   concrete &                  energy &                          naval \\
Algorithm & Prior& (506, 13, 1)& (10721, 5, 3)& (1030, 8, 1)& (768, 8, 2)& (11934, 16, 2)\\
\midrule
Detlefsen & N/A &           -0.67$\pm$1.81 &          -9.8e-04$\pm$3.5e-03 &             -0.03$\pm$3.30 &           0.15$\pm$0.87 &           -2.8e-04$\pm$6.3e-04 \\
Normal & N/A &           -0.28$\pm$0.56 &           5.5e-05$\pm$2.1e-04 &              0.32$\pm$0.66 &           0.06$\pm$0.10 &           -1.3e-04$\pm$1.2e-04 \\
Student & N/A &           -0.50$\pm$0.51 &          -4.3e-05$\pm$1.4e-04 &             -0.04$\pm$0.72 &          -0.06$\pm$0.13 &           -1.0e-04$\pm$1.5e-04 \\
Gamma-Normal & VAP &           -0.31$\pm$0.54 &           1.5e-04$\pm$2.2e-04 &              0.06$\pm$0.73 &          -0.03$\pm$0.12 &           -4.1e-05$\pm$8.1e-05 \\
             & Standard &           -0.39$\pm$0.67 &           5.0e-05$\pm$1.9e-04 &              0.09$\pm$0.72 &           0.04$\pm$0.10 &           -1.4e-04$\pm$8.5e-05 \\
             & VAMP &  \textbf{-0.18$\pm$0.52} &  \textbf{9.5e-06$\pm$2.3e-04} &             -0.10$\pm$0.58 &  \textbf{0.02$\pm$0.11} &           -4.6e-06$\pm$5.5e-05 \\
             & VAMP* &           -0.18$\pm$0.52 &           7.9e-05$\pm$2.0e-04 &             -0.10$\pm$0.58 &           0.02$\pm$0.11 &           -8.9e-06$\pm$6.0e-05 \\
             & xVAMP &           -0.25$\pm$0.54 &           4.6e-05$\pm$1.8e-04 &  \textbf{9.2e-03$\pm$0.63} &           0.03$\pm$0.11 &  \textbf{-1.8e-06$\pm$7.1e-05} \\
             & xVAMP* &           -0.24$\pm$0.54 &           1.3e-04$\pm$2.0e-04 &              0.03$\pm$0.66 &           0.02$\pm$0.11 &            3.8e-06$\pm$6.2e-05 \\
             & VBEM &           -0.18$\pm$0.54 &           7.3e-05$\pm$3.8e-04 &             -0.01$\pm$0.55 &           0.03$\pm$0.11 &            1.5e-05$\pm$2.8e-05 \\
             & VBEM* &           -0.19$\pm$0.58 &          -2.2e-05$\pm$2.1e-04 &             -0.02$\pm$0.63 &           0.03$\pm$0.11 &            1.9e-05$\pm$5.8e-05 \\
\midrule
             &       &                power plant &       superconductivity &                    wine-red &                 wine-white &                    yacht \\
Algorithm & Prior& (9568, 4, 1)& (21263, 81, 1)& (1599, 11, 1)& (4898, 11, 1)& (308, 6, 1)\\
\midrule
Detlefsen & N/A &              0.15$\pm$0.79 &           1.22$\pm$3.11 &               0.02$\pm$0.12 &  \textbf{2.8e-03$\pm$0.08} &  \textbf{-0.06$\pm$1.19} \\
Normal & N/A &          -9.9e-03$\pm$0.07 &           0.90$\pm$0.62 &  \textbf{-5.1e-03$\pm$0.06} &          -3.3e-03$\pm$0.03 &           -0.96$\pm$0.82 \\
Student & N/A &              0.06$\pm$0.08 &           0.29$\pm$0.54 &              -0.07$\pm$0.06 &             -0.02$\pm$0.03 &           -7.47$\pm$2.71 \\
Gamma-Normal & VAP &              0.02$\pm$0.05 &          -0.08$\pm$0.33 &              -0.01$\pm$0.06 &          -7.0e-03$\pm$0.03 &           -7.22$\pm$2.74 \\
             & Standard &          -9.6e-03$\pm$0.11 &           0.74$\pm$0.33 &              -0.02$\pm$0.06 &             -0.01$\pm$0.03 &           -5.42$\pm$1.86 \\
             & VAMP &           3.2e-03$\pm$0.06 &           0.09$\pm$0.38 &              -0.01$\pm$0.06 &             -0.01$\pm$0.03 &           -0.62$\pm$1.53 \\
             & VAMP* &           3.2e-03$\pm$0.06 &           0.06$\pm$0.39 &              -0.01$\pm$0.06 &             -0.01$\pm$0.03 &           -0.60$\pm$1.53 \\
             & xVAMP &           6.5e-03$\pm$0.07 &          -0.03$\pm$0.41 &           -9.6e-03$\pm$0.06 &          -7.9e-03$\pm$0.03 &           -5.44$\pm$2.46 \\
             & xVAMP* &           2.0e-03$\pm$0.06 &  \textbf{0.01$\pm$0.49} &           -8.8e-03$\pm$0.06 &          -8.7e-03$\pm$0.03 &           -5.59$\pm$2.61 \\
             & VBEM &           1.2e-03$\pm$0.10 &           0.25$\pm$0.45 &           -9.6e-03$\pm$0.06 &          -5.8e-03$\pm$0.03 &           -0.17$\pm$0.52 \\
             & VBEM* &  \textbf{3.0e-05$\pm$0.07} &           0.09$\pm$0.46 &           -9.2e-03$\pm$0.06 &          -7.6e-03$\pm$0.02 &           -2.00$\pm$1.30 \\
\bottomrule
\end{tabular}

}
    \end{center}
\end{table}

\begin{table}[ht!]
    \caption{UCI Mean RMSE \meanpmstd \ \tuple}
    \label{tab:uci-mean-RMSE}
    \begin{center}
	    {\scriptsize \begin{tabular}{lllllll}
\toprule
             &       &                  boston &                        carbon &                concrete &                  energy &                         naval \\
Algorithm & Prior& (506, 13, 1)& (10721, 5, 3)& (1030, 8, 1)& (768, 8, 2)& (11934, 16, 2)\\
\midrule
\cite{sun2019functional} & N/A & \textit{2.38$\pm$0.10} & -- & \textit{4.94$\pm$0.18} & \textit{0.41$\pm$0.02} & \textit{1.2e-04$\pm$0.00} \\
Detlefsen & N/A &           4.48$\pm$1.06 &              0.02$\pm$4.6e-03 &           8.13$\pm$1.65 &           2.05$\pm$0.49 &           4.2e-03$\pm$6.3e-04 \\
Normal & N/A &           3.36$\pm$1.29 &  \textbf{7.5e-03$\pm$3.3e-03} &           6.05$\pm$0.66 &           1.30$\pm$0.14 &           3.5e-03$\pm$3.1e-04 \\
Student & N/A &           3.62$\pm$1.42 &           7.6e-03$\pm$3.3e-03 &           6.71$\pm$0.81 &           1.42$\pm$0.17 &           3.4e-03$\pm$5.0e-04 \\
Gamma-Normal & VAP &           3.44$\pm$1.21 &           7.7e-03$\pm$3.3e-03 &           6.61$\pm$0.84 &           1.38$\pm$0.15 &           3.2e-03$\pm$5.3e-04 \\
             & Standard &           3.82$\pm$1.72 &           7.6e-03$\pm$3.3e-03 &           6.63$\pm$0.70 &           1.31$\pm$0.14 &           3.2e-03$\pm$5.1e-04 \\
             & VAMP &           3.15$\pm$1.06 &           7.8e-03$\pm$3.2e-03 &           5.47$\pm$1.00 &           1.36$\pm$0.13 &           1.2e-03$\pm$1.0e-03 \\
             & VAMP* &           3.15$\pm$1.05 &           7.8e-03$\pm$3.2e-03 &           5.47$\pm$1.00 &           1.36$\pm$0.13 &           1.6e-03$\pm$1.3e-03 \\
             & xVAMP &           3.25$\pm$1.16 &           7.6e-03$\pm$3.3e-03 &           5.61$\pm$0.67 &           1.36$\pm$0.14 &           3.2e-03$\pm$5.2e-04 \\
             & xVAMP* &           3.28$\pm$1.17 &           7.6e-03$\pm$3.3e-03 &           5.72$\pm$0.59 &           1.36$\pm$0.14 &           3.2e-03$\pm$4.9e-04 \\
             & VBEM &  \textbf{3.14$\pm$1.07} &           8.7e-03$\pm$3.3e-03 &  \textbf{5.26$\pm$0.58} &           1.36$\pm$0.14 &  \textbf{5.6e-04$\pm$1.6e-04} \\
             & VBEM* &           3.18$\pm$1.12 &           7.6e-03$\pm$3.3e-03 &           5.59$\pm$0.70 &  \textbf{1.30$\pm$0.13} &           2.4e-03$\pm$2.8e-04 \\
\midrule
             &       &             power plant &        superconductivity &                wine-red &              wine-white &                   yacht \\
Algorithm & Prior& (9568, 4, 1)& (21263, 81, 1)& (1599, 11, 1)& (4898, 11, 1)& (308, 6, 1)\\
\midrule
\cite{sun2019functional} & N/A & \textit{4.10$\pm$0.05} & -- & -- & -- & \textit{0.61$\pm$0.07} \\
Detlefsen & N/A &           4.33$\pm$0.27 &           17.72$\pm$1.29 &           0.71$\pm$0.06 &           0.76$\pm$0.04 &  \textbf{2.42$\pm$1.06} \\
Normal & N/A &  \textbf{4.12$\pm$0.20} &           14.53$\pm$0.44 &           0.62$\pm$0.03 &           0.70$\pm$0.04 &           3.42$\pm$2.30 \\
Student & N/A &           4.12$\pm$0.19 &           14.85$\pm$0.42 &           0.63$\pm$0.03 &           0.71$\pm$0.03 &          15.03$\pm$3.30 \\
Gamma-Normal & VAP &           4.14$\pm$0.21 &           14.83$\pm$0.48 &           0.62$\pm$0.03 &           0.70$\pm$0.03 &          14.70$\pm$3.31 \\
             & Standard &           4.18$\pm$0.18 &           14.44$\pm$0.43 &           0.63$\pm$0.03 &           0.72$\pm$0.03 &          12.17$\pm$2.38 \\
             & VAMP &           4.16$\pm$0.20 &           12.81$\pm$0.33 &           0.62$\pm$0.03 &           0.70$\pm$0.04 &           5.42$\pm$3.54 \\
             & VAMP* &           4.16$\pm$0.20 &  \textbf{12.80$\pm$0.35} &           0.62$\pm$0.03 &           0.70$\pm$0.04 &           5.30$\pm$3.65 \\
             & xVAMP &           4.14$\pm$0.20 &           14.13$\pm$0.39 &           0.62$\pm$0.03 &           0.70$\pm$0.04 &          12.30$\pm$3.09 \\
             & xVAMP* &           4.13$\pm$0.21 &           14.25$\pm$0.42 &           0.62$\pm$0.03 &           0.70$\pm$0.03 &          12.51$\pm$3.20 \\
             & VBEM &           4.16$\pm$0.19 &           13.13$\pm$0.37 &  \textbf{0.62$\pm$0.03} &  \textbf{0.69$\pm$0.03} &           3.51$\pm$1.46 \\
             & VBEM* &           4.12$\pm$0.19 &           14.08$\pm$0.42 &           0.62$\pm$0.03 &           0.69$\pm$0.03 &           5.33$\pm$2.58 \\
\bottomrule
\end{tabular}

}
    \end{center}
\end{table}

\begin{table}[ht!]
    \caption{UCI Variance Bias \meanpmstd \ \tuple}
    \label{tab:uci-var-bias}
    \begin{center}
	    {\scriptsize \begin{tabular}{lllllll}
\toprule
             &       &                   boston &                         carbon &                 concrete &                     energy &                         naval \\
Algorithm & Prior& (506, 13, 1)& (10721, 5, 3)& (1030, 8, 1)& (768, 8, 2)& (11934, 16, 2)\\
\midrule
Detlefsen & N/A &        1.0e+02$\pm$79.11 &            9.8e-05$\pm$1.6e-04 &        2.2e+02$\pm$91.85 &             18.60$\pm$8.88 &                   nan$\pm$nan \\
Normal & N/A &        31.63$\pm$1.5e+02 &            3.5e+23$\pm$1.6e+24 &           -2.01$\pm$8.67 &             -0.16$\pm$0.24 &           3.1e-07$\pm$2.0e-06 \\
Student & N/A &          18.08$\pm$63.79 &                  0.12$\pm$0.23 &           -2.20$\pm$9.28 &            24.00$\pm$85.42 &           4.9e-06$\pm$2.2e-05 \\
Gamma-Normal & VAP &      3.3e+02$\pm$1.3e+03 &                  0.25$\pm$1.11 &           -2.13$\pm$7.85 &              0.04$\pm$0.31 &           3.1e-07$\pm$6.8e-07 \\
             & Standard &           3.18$\pm$20.09 &            1.5e-04$\pm$5.8e-05 &           0.76$\pm$11.35 &              0.31$\pm$0.40 &           3.7e-06$\pm$2.9e-06 \\
             & VAMP &           -2.96$\pm$7.96 &           -6.6e-06$\pm$6.0e-05 &           -6.15$\pm$5.18 &             -0.15$\pm$0.39 &           1.7e-07$\pm$2.9e-07 \\
             & VAMP* &           -3.00$\pm$7.84 &  \textbf{-6.0e-06$\pm$6.0e-05} &           -6.16$\pm$5.18 &             -0.13$\pm$0.40 &  \textbf{1.3e-07$\pm$3.3e-07} \\
             & xVAMP &           0.65$\pm$16.20 &            2.7e-05$\pm$9.7e-05 &           -4.82$\pm$4.63 &  \textbf{6.0e-03$\pm$0.36} &           3.1e-07$\pm$7.4e-07 \\
             & xVAMP* &           0.51$\pm$20.17 &            5.0e-04$\pm$2.2e-03 &           -4.66$\pm$5.07 &          -8.5e-03$\pm$0.36 &           2.7e-07$\pm$6.3e-07 \\
             & VBEM &            6.74$\pm$8.48 &               0.01$\pm$4.5e-03 &           25.86$\pm$8.94 &             22.06$\pm$5.58 &           3.6e-05$\pm$1.4e-05 \\
             & VBEM* &  \textbf{-0.11$\pm$8.62} &           -7.2e-06$\pm$6.1e-05 &  \textbf{-0.58$\pm$5.05} &              0.02$\pm$0.28 &           3.9e-07$\pm$4.9e-07 \\
\midrule
             &       &             power plant &        superconductivity &                   wine-red &                  wine-white &                     yacht \\
Algorithm & Prior& (9568, 4, 1)& (21263, 81, 1)& (1599, 11, 1)& (4898, 11, 1)& (308, 6, 1)\\
\midrule
Detlefsen & N/A &          69.25$\pm$2.40 &      5.5e+04$\pm$6.2e+03 &              2.16$\pm$1.57 &               0.83$\pm$0.36 &           96.62$\pm$54.08 \\
Normal & N/A &  \textbf{0.05$\pm$1.53} &      2.3e+13$\pm$1.0e+14 &          -3.8e-03$\pm$0.04 &              -0.02$\pm$0.06 &           20.68$\pm$54.95 \\
Student & N/A &          -0.27$\pm$1.47 &      1.6e+05$\pm$3.3e+05 &            12.52$\pm$30.71 &           -5.6e-03$\pm$0.05 &       1.7e+03$\pm$2.3e+03 \\
Gamma-Normal & VAP &           0.52$\pm$1.29 &      9.0e+05$\pm$2.6e+06 &              0.03$\pm$0.05 &               0.13$\pm$0.64 &       1.3e+03$\pm$1.5e+03 \\
             & Standard &           2.34$\pm$1.43 &        1.1e+02$\pm$81.21 &              0.04$\pm$0.11 &  \textbf{-2.3e-03$\pm$0.05} &  \textbf{-7.28$\pm$40.88} \\
             & VAMP &           0.89$\pm$1.04 &  \textbf{-9.83$\pm$7.97} &              0.05$\pm$0.06 &           -8.8e-03$\pm$0.04 &           38.05$\pm$83.39 \\
             & VAMP* &           0.89$\pm$1.04 &           -9.89$\pm$7.98 &              0.05$\pm$0.06 &           -8.9e-03$\pm$0.04 &           38.07$\pm$83.29 \\
             & xVAMP &           0.46$\pm$1.25 &          14.40$\pm$42.90 &           3.5e-03$\pm$0.05 &              -0.03$\pm$0.03 &       4.8e+02$\pm$1.7e+03 \\
             & xVAMP* &           0.44$\pm$1.24 &      1.3e+02$\pm$4.7e+02 &  \textbf{2.1e-03$\pm$0.05} &              -0.03$\pm$0.03 &       1.7e+02$\pm$1.5e+02 \\
             & VBEM &          16.53$\pm$9.32 &          91.44$\pm$25.39 &              0.08$\pm$0.04 &               0.07$\pm$0.04 &           20.70$\pm$25.23 \\
             & VBEM* &           1.86$\pm$1.44 &           9.87$\pm$16.22 &              0.05$\pm$0.06 &               0.01$\pm$0.04 &           26.48$\pm$26.88 \\
\bottomrule
\end{tabular}

}
    \end{center}
\end{table}

\begin{table}[ht!]
    \caption{UCI Variance RMSE \meanpmstd \ \tuple}
    \label{tab:uci-var-RMSE}
    \begin{center}
	    {\scriptsize \begin{tabular}{lllllll}
\toprule
             &       &                    boston &                        carbon &                  concrete &                  energy &                         naval \\
Algorithm & Prior& (506, 13, 1)& (10721, 5, 3)& (1030, 8, 1)& (768, 8, 2)& (11934, 16, 2)\\
\midrule
Detlefsen & N/A &       2.5e+02$\pm$3.1e+02 &           2.8e-03$\pm$1.8e-03 &       2.9e+02$\pm$1.1e+02 &         21.58$\pm$10.55 &                   nan$\pm$nan \\
Normal & N/A &       2.8e+02$\pm$1.1e+03 &           2.0e+25$\pm$8.8e+25 &           84.48$\pm$46.55 &  \textbf{2.70$\pm$0.50} &           3.6e-05$\pm$1.5e-05 \\
Student & N/A &       1.1e+02$\pm$1.7e+02 &                 1.19$\pm$2.12 &           86.73$\pm$25.52 &     1.0e+02$\pm$3.6e+02 &           1.4e-04$\pm$4.8e-04 \\
Gamma-Normal & VAP &       2.4e+03$\pm$9.5e+03 &                4.74$\pm$20.81 &           80.57$\pm$26.95 &           3.64$\pm$1.10 &           2.3e-05$\pm$8.7e-06 \\
             & Standard &           76.10$\pm$83.67 &           2.8e-03$\pm$1.8e-03 &           92.78$\pm$28.09 &           3.05$\pm$1.00 &           3.0e-05$\pm$1.1e-05 \\
             & VAMP &           31.89$\pm$37.72 &  \textbf{2.7e-03$\pm$1.9e-03} &           60.50$\pm$29.84 &           4.19$\pm$0.79 &  \textbf{5.5e-06$\pm$7.0e-06} \\
             & VAMP* &  \textbf{31.82$\pm$37.33} &           2.7e-03$\pm$1.9e-03 &           60.49$\pm$29.84 &           4.19$\pm$0.79 &           7.8e-06$\pm$9.1e-06 \\
             & xVAMP &           63.40$\pm$84.86 &           3.0e-03$\pm$1.7e-03 &           59.74$\pm$20.73 &           3.36$\pm$0.88 &           2.3e-05$\pm$8.7e-06 \\
             & xVAMP* &         64.27$\pm$1.2e+02 &                 0.02$\pm$0.05 &           62.39$\pm$19.00 &           3.19$\pm$0.78 &           2.2e-05$\pm$6.3e-06 \\
             & VBEM &           38.91$\pm$35.36 &              0.01$\pm$4.3e-03 &           59.36$\pm$13.87 &          26.09$\pm$6.92 &           4.2e-05$\pm$1.6e-05 \\
             & VBEM* &           39.54$\pm$42.93 &           2.8e-03$\pm$1.9e-03 &  \textbf{58.92$\pm$19.43} &           3.72$\pm$0.47 &           1.5e-05$\pm$3.8e-06 \\
\midrule
             &       &               power plant &           superconductivity &                wine-red &              wine-white &                     yacht \\
Algorithm & Prior& (9568, 4, 1)& (21263, 81, 1)& (1599, 11, 1)& (4898, 11, 1)& (308, 6, 1)\\
\midrule
Detlefsen & N/A &           85.20$\pm$10.25 &         2.2e+05$\pm$1.7e+04 &           7.27$\pm$9.73 &           2.91$\pm$3.65 &         1.1e+02$\pm$70.70 \\
Normal & N/A &  \textbf{43.93$\pm$18.42} &         1.1e+15$\pm$4.8e+15 &           0.63$\pm$0.09 &           1.05$\pm$0.82 &       1.2e+02$\pm$2.7e+02 \\
Student & N/A &           44.88$\pm$18.75 &         5.8e+06$\pm$1.3e+07 &     1.2e+02$\pm$3.4e+02 &           0.96$\pm$0.35 &       5.7e+03$\pm$8.2e+03 \\
Gamma-Normal & VAP &           44.40$\pm$18.82 &         4.0e+07$\pm$1.2e+08 &           0.65$\pm$0.10 &          3.97$\pm$13.91 &       4.8e+03$\pm$5.7e+03 \\
             & Standard &           45.18$\pm$18.49 &         1.5e+03$\pm$1.7e+03 &           0.77$\pm$0.38 &           0.94$\pm$0.20 &         1.1e+02$\pm$66.59 \\
             & VAMP &           44.78$\pm$18.79 &  \textbf{4.4e+02$\pm$55.55} &           0.63$\pm$0.09 &           0.87$\pm$0.25 &         99.44$\pm$1.2e+02 \\
             & VAMP* &           44.78$\pm$18.79 &           4.4e+02$\pm$57.11 &           0.63$\pm$0.09 &           0.87$\pm$0.25 &         98.63$\pm$1.3e+02 \\
             & xVAMP &           44.44$\pm$18.84 &         1.1e+03$\pm$1.8e+03 &  \textbf{0.63$\pm$0.11} &           0.85$\pm$0.23 &       1.4e+03$\pm$4.8e+03 \\
             & xVAMP* &           44.36$\pm$18.82 &         6.4e+03$\pm$2.1e+04 &           0.63$\pm$0.11 &           0.85$\pm$0.23 &       5.6e+02$\pm$4.9e+02 \\
             & VBEM &           49.60$\pm$16.88 &           4.5e+02$\pm$59.88 &           0.63$\pm$0.11 &  \textbf{0.82$\pm$0.11} &  \textbf{39.19$\pm$37.73} \\
             & VBEM* &           44.68$\pm$18.61 &         6.3e+02$\pm$4.2e+02 &           0.64$\pm$0.10 &           0.86$\pm$0.28 &           93.02$\pm$86.57 \\
\bottomrule
\end{tabular}

}
    \end{center}
\end{table}

\begin{table}[ht!]
    \caption{UCI Sample Bias \meanpmstd \ \tuple}
    \label{tab:uci-samp-bias}
    \begin{center}
	    {\scriptsize \begin{tabular}{lllllll}
\toprule
             &       &                   boston &                         carbon &                 concrete &                     energy &                          naval \\
Algorithm & Prior& (506, 13, 1)& (10721, 5, 3)& (1030, 8, 1)& (768, 8, 2)& (11934, 16, 2)\\
\midrule
Detlefsen & N/A &           -0.92$\pm$2.52 &           -9.4e-04$\pm$3.6e-03 &            0.49$\pm$3.93 &              0.17$\pm$1.03 &           -2.6e-04$\pm$6.1e-04 \\
Normal & N/A &  \textbf{-0.19$\pm$0.99} &            4.6e+09$\pm$2.0e+10 &            0.39$\pm$1.05 &              0.06$\pm$0.15 &           -1.2e-04$\pm$1.4e-04 \\
Student & N/A &           -0.58$\pm$0.60 &           -4.3e-05$\pm$1.5e-04 &           -0.14$\pm$1.09 &             -0.07$\pm$0.15 &           -8.3e-05$\pm$2.0e-04 \\
Gamma-Normal & VAP &           -0.34$\pm$0.54 &            1.5e-04$\pm$2.1e-04 &  \textbf{-0.02$\pm$1.18} &             -0.04$\pm$0.14 &  \textbf{-7.0e-06$\pm$1.1e-04} \\
             & Standard &           -0.39$\pm$0.59 &            7.2e-05$\pm$2.9e-04 &            0.04$\pm$1.02 &              0.04$\pm$0.13 &           -1.3e-04$\pm$1.2e-04 \\
             & VAMP &           -0.23$\pm$0.47 &  \textbf{-1.8e-06$\pm$2.9e-04} &           -0.17$\pm$0.83 &              0.01$\pm$0.12 &            7.4e-06$\pm$5.5e-05 \\
             & VAMP* &           -0.24$\pm$0.47 &            6.7e-05$\pm$2.7e-04 &           -0.17$\pm$0.83 &              0.02$\pm$0.12 &            8.2e-06$\pm$5.9e-05 \\
             & xVAMP &           -0.23$\pm$0.69 &           -1.8e-05$\pm$2.4e-04 &           -0.08$\pm$0.88 &           6.0e-03$\pm$0.16 &           -2.2e-05$\pm$1.2e-04 \\
             & xVAMP* &           -0.23$\pm$0.68 &            7.9e-05$\pm$2.6e-04 &           -0.09$\pm$0.97 &  \textbf{2.6e-03$\pm$0.15} &           -1.8e-05$\pm$1.2e-04 \\
             & VBEM &           -0.19$\pm$0.85 &           -4.2e-04$\pm$2.0e-03 &           -0.15$\pm$1.07 &             -0.09$\pm$0.49 &           -2.3e-05$\pm$1.4e-04 \\
             & VBEM* &           -0.24$\pm$0.70 &            3.3e-06$\pm$3.0e-04 &            0.02$\pm$0.79 &              0.02$\pm$0.10 &            1.8e-05$\pm$6.8e-05 \\
\midrule
             &       &                 power plant &       superconductivity &                   wine-red &                  wine-white &                    yacht \\
Algorithm & Prior& (9568, 4, 1)& (21263, 81, 1)& (1599, 11, 1)& (4898, 11, 1)& (308, 6, 1)\\
\midrule
Detlefsen & N/A &               0.12$\pm$0.77 &           1.15$\pm$4.61 &              0.07$\pm$0.18 &           -4.9e-03$\pm$0.08 &           -0.19$\pm$2.16 \\
Normal & N/A &               0.02$\pm$0.16 &     3.6e+04$\pm$1.6e+05 &  \textbf{1.7e-03$\pm$0.08} &            3.8e-03$\pm$0.05 &           -0.70$\pm$1.15 \\
Student & N/A &               0.04$\pm$0.13 &           0.29$\pm$0.61 &             -0.07$\pm$0.08 &              -0.03$\pm$0.04 &           -6.26$\pm$4.34 \\
Gamma-Normal & VAP &  \textbf{-7.6e-03$\pm$0.15} &          -0.06$\pm$0.41 &             -0.02$\pm$0.08 &              -0.02$\pm$0.04 &           -6.16$\pm$4.37 \\
             & Standard &              -0.04$\pm$0.16 &           0.70$\pm$0.51 &             -0.03$\pm$0.08 &              -0.02$\pm$0.04 &           -4.92$\pm$2.49 \\
             & VAMP &              -0.02$\pm$0.13 &           0.16$\pm$0.46 &             -0.02$\pm$0.08 &              -0.02$\pm$0.04 &           -0.62$\pm$1.94 \\
             & VAMP* &              -0.02$\pm$0.13 &           0.14$\pm$0.45 &             -0.02$\pm$0.08 &              -0.02$\pm$0.04 &           -0.58$\pm$1.94 \\
             & xVAMP &              -0.02$\pm$0.18 &          -0.16$\pm$0.62 &             -0.02$\pm$0.08 &              -0.02$\pm$0.04 &           -5.13$\pm$2.98 \\
             & xVAMP* &              -0.02$\pm$0.15 &          -0.13$\pm$0.62 &             -0.02$\pm$0.08 &              -0.02$\pm$0.04 &           -5.36$\pm$3.12 \\
             & VBEM &              -0.04$\pm$0.21 &           0.10$\pm$0.67 &             -0.02$\pm$0.08 &              -0.01$\pm$0.04 &  \textbf{-0.19$\pm$0.89} \\
             & VBEM* &               0.04$\pm$0.15 &  \textbf{0.04$\pm$0.57} &          -7.3e-03$\pm$0.06 &  \textbf{-2.3e-03$\pm$0.04} &           -1.74$\pm$1.59 \\
\bottomrule
\end{tabular}

}
    \end{center}
\end{table}

\clearpage
\begin{table}[ht!]
    \caption{UCI Sample RMSE \meanpmstd \ \tuple}
    \label{tab:uci-samp-RMSE}
    \begin{center}
	    {\scriptsize \begin{tabular}{lllllll}
\toprule
             &       &                  boston &                        carbon &                concrete &                  energy &                         naval \\
Algorithm & Prior& (506, 13, 1)& (10721, 5, 3)& (1030, 8, 1)& (768, 8, 2)& (11934, 16, 2)\\
\midrule
Detlefsen & N/A &          12.02$\pm$3.89 &              0.03$\pm$3.6e-03 &          17.93$\pm$2.55 &           5.07$\pm$0.98 &           6.2e-03$\pm$5.7e-04 \\
Normal & N/A &           4.92$\pm$3.57 &           2.6e+11$\pm$1.2e+12 &           8.23$\pm$1.08 &  \textbf{1.85$\pm$0.21} &           5.0e-03$\pm$5.4e-04 \\
Student & N/A &           4.64$\pm$1.10 &  \textbf{8.1e-03$\pm$3.1e-03} &           9.18$\pm$1.36 &           2.07$\pm$0.37 &           5.0e-03$\pm$1.7e-03 \\
Gamma-Normal & VAP &           4.69$\pm$0.86 &              0.01$\pm$2.2e-03 &           9.42$\pm$1.82 &           2.02$\pm$0.35 &           4.5e-03$\pm$7.2e-04 \\
             & Standard &           4.92$\pm$2.18 &              0.02$\pm$1.8e-03 &           8.67$\pm$1.20 &           1.88$\pm$0.38 &           4.6e-03$\pm$9.1e-04 \\
             & VAMP &           4.27$\pm$0.87 &              0.01$\pm$1.9e-03 &           7.27$\pm$1.05 &           1.93$\pm$0.19 &  \textbf{1.8e-03$\pm$1.4e-03} \\
             & VAMP* &           4.26$\pm$0.86 &              0.01$\pm$2.0e-03 &  \textbf{7.27$\pm$1.05} &           1.93$\pm$0.20 &           2.2e-03$\pm$1.8e-03 \\
             & xVAMP &  \textbf{4.23$\pm$1.15} &              0.01$\pm$2.0e-03 &           7.84$\pm$1.05 &           1.88$\pm$0.29 &           4.5e-03$\pm$7.5e-04 \\
             & xVAMP* &           4.23$\pm$1.14 &              0.01$\pm$2.5e-03 &           8.00$\pm$1.01 &           1.87$\pm$0.30 &           4.5e-03$\pm$7.1e-04 \\
             & VBEM &           5.03$\pm$0.92 &                 0.11$\pm$0.03 &           9.21$\pm$0.98 &           5.13$\pm$0.83 &           5.9e-03$\pm$1.5e-03 \\
             & VBEM* &           4.41$\pm$1.07 &              0.01$\pm$1.9e-03 &           7.90$\pm$1.10 &           1.85$\pm$0.30 &           3.5e-03$\pm$3.7e-04 \\
\midrule
             &       &             power plant &        superconductivity &                wine-red &              wine-white &                   yacht \\
Algorithm & Prior& (9568, 4, 1)& (21263, 81, 1)& (1599, 11, 1)& (4898, 11, 1)& (308, 6, 1)\\
\midrule
Detlefsen & N/A &          10.36$\pm$0.28 &        2.4e+02$\pm$15.98 &           1.43$\pm$0.34 &           1.27$\pm$0.10 &          10.71$\pm$2.19 \\
Normal & N/A &           5.85$\pm$0.20 &      1.7e+06$\pm$7.4e+06 &  \textbf{0.86$\pm$0.07} &           0.98$\pm$0.03 &  \textbf{4.73$\pm$3.68} \\
Student & N/A &  \textbf{5.79$\pm$0.28} &           21.25$\pm$1.46 &           0.88$\pm$0.06 &           0.99$\pm$0.04 &          20.24$\pm$7.84 \\
Gamma-Normal & VAP &           5.90$\pm$0.26 &           21.05$\pm$0.81 &           0.89$\pm$0.06 &           0.99$\pm$0.04 &          20.00$\pm$7.47 \\
             & Standard &           6.01$\pm$0.51 &          23.75$\pm$13.27 &           0.90$\pm$0.13 &           0.98$\pm$0.06 &          14.20$\pm$4.40 \\
             & VAMP &           5.97$\pm$0.28 &           17.86$\pm$0.41 &           0.90$\pm$0.07 &           0.99$\pm$0.06 &           8.67$\pm$6.43 \\
             & VAMP* &           5.97$\pm$0.28 &  \textbf{17.85$\pm$0.42} &           0.90$\pm$0.07 &           0.99$\pm$0.06 &           8.50$\pm$6.57 \\
             & xVAMP &           5.92$\pm$0.20 &           19.98$\pm$0.49 &           0.89$\pm$0.05 &  \textbf{0.97$\pm$0.06} &          15.57$\pm$5.76 \\
             & xVAMP* &           5.91$\pm$0.20 &           20.19$\pm$0.77 &           0.89$\pm$0.05 &           0.97$\pm$0.06 &          15.81$\pm$5.05 \\
             & VBEM &           7.17$\pm$0.65 &           20.92$\pm$0.70 &           0.93$\pm$0.06 &           1.02$\pm$0.05 &           6.66$\pm$2.53 \\
             & VBEM* &           6.00$\pm$0.20 &           19.78$\pm$0.48 &           0.89$\pm$0.07 &           0.97$\pm$0.03 &           6.84$\pm$4.58 \\
\bottomrule
\end{tabular}

}
    \end{center}
\end{table}

\section{Variational Variance for VAEs}
For the VAE experiments, we use ADAM with a 5e-5 learning rate. All Monte-Carlo (MC) approximations use 20 samples. We found additional samples did not improve log posterior predictive probability approximations. Since our VAMP($^*$), xVAMP($^*$), and VBEM$^*$ priors require twice as many MC samples ($q(\lambda|x)$ in addition to $q(z|x)$), their memory footprint is higher, requiring a batch size of 125 on a NVIDA RTX2070. The remaining models use a batch size of 256. Because the lower batch size has twice as many batch updates per epoch, those models train for half (500) the number of epochs used by the other models (1000). We employ early stopping on the validation set's log posterior predictive probability with a patience of 25 for the 500 epoch models and 50 for the 1000 epoch models. We use an encoder architecture with hidden layers of sizes 512, 256, and 128, each of which applies an ELU activation. The decoder architecture is the transpose of the encoder. The dimensions of the latent variable, $\dim(z)$, are 10 for MNIST and 25 for Fashion MNIST.

We include PPC metrics for MNIST in \cref{tab:vae-mnist}, which we could not fit in the main report. Additionally, we include \cref{fig:fashion,fig:mnist}, which are similar to fig. 3 (main article) but have additional samples for \emph{all} tested methods.
\begin{table}[H]
    \caption{VAE PPCs for MNIST \meanpmstd}
    \label{tab:vae-mnist}
    \begin{center}
	    {\scriptsize \begin{tabular}{lllll}
\toprule
{} &                           LL &                  Mean RMSE &                      Var Bias &                Sample RMSE \\
Method                 &                              &                            &                               &                            \\
\midrule
Fixed-Var. VAE (1.0)   &             -732.10$\pm$0.11 &           0.17$\pm$1.1e-03 &              0.98$\pm$4.2e-04 &           1.02$\pm$2.5e-04 \\
Fixed-Var. VAE (0.001) &           -2902.66$\pm$29.23 &  \textbf{0.11$\pm$3.3e-04} &          -1.2e-02$\pm$7.4e-05 &  \textbf{0.12$\pm$3.1e-04} \\
VAE                    &           2593.51$\pm$267.72 &           0.25$\pm$2.7e-03 &           4.3e-02$\pm$2.6e-02 &           0.41$\pm$3.5e-02 \\
VAE + BN               &            2386.70$\pm$23.17 &           0.25$\pm$1.8e-03 &              0.13$\pm$2.6e-02 &           0.50$\pm$2.6e-02 \\
VAE-Split              &            2282.32$\pm$65.63 &           0.25$\pm$2.7e-03 &           7.4e-02$\pm$2.6e-02 &           0.44$\pm$3.2e-02 \\
VAE-Split + BN         &            2482.36$\pm$75.34 &           0.28$\pm$4.4e-03 &           6.2e-02$\pm$1.1e-02 &           0.47$\pm$1.5e-02 \\
Detlefsen              &            -1561.89$\pm$1.36 &           0.18$\pm$6.7e-04 &              9.12$\pm$2.1e-02 &           3.03$\pm$3.2e-03 \\
MAP-VAE                &             1291.42$\pm$6.94 &           0.13$\pm$1.9e-03 &          -1.3e-02$\pm$4.1e-04 &           0.15$\pm$2.0e-03 \\
Student-VAE            &  \textbf{4826.82$\pm$530.95} &           0.27$\pm$1.7e-02 &                 0.38$\pm$0.45 &              0.68$\pm$0.28 \\
V3AE-VAP               &           3243.11$\pm$445.47 &           0.24$\pm$3.5e-03 &  \textbf{8.1e-04$\pm$9.7e-04} &           0.34$\pm$5.5e-03 \\
V3AE-Gamma             &             1495.01$\pm$2.75 &           0.13$\pm$7.0e-04 &          -1.2e-02$\pm$1.9e-04 &           0.15$\pm$9.2e-04 \\
V3AE-VAMP              &            2355.12$\pm$13.40 &           0.20$\pm$6.7e-04 &  \textbf{6.2e-04$\pm$1.1e-03} &           0.28$\pm$1.7e-03 \\
V3AE-VAMP*             &            2270.76$\pm$41.89 &           0.20$\pm$7.9e-04 &  \textbf{1.2e-03$\pm$1.1e-03} &           0.29$\pm$2.2e-03 \\
V3AE-xVAMP             &            2323.38$\pm$94.35 &           0.20$\pm$2.6e-03 &  \textbf{1.9e-03$\pm$6.8e-04} &           0.29$\pm$3.2e-03 \\
V3AE-xVAMP*            &            2280.13$\pm$48.29 &           0.20$\pm$2.0e-03 &  \textbf{6.5e-04$\pm$7.2e-04} &           0.29$\pm$3.7e-03 \\
V3AE-VBEM              &              296.95$\pm$0.92 &           0.12$\pm$8.1e-04 &           6.1e-02$\pm$2.7e-04 &           0.30$\pm$2.7e-04 \\
V3AE-VBEM*             &             2107.63$\pm$5.44 &           0.14$\pm$1.2e-03 &  \textbf{1.6e-03$\pm$1.1e-04} &           0.20$\pm$1.6e-03 \\
\bottomrule
\end{tabular}

}
    \end{center}
\end{table}

\clearpage
\begin{figure}
    \centering
    \includegraphics[height=0.9\textheight]{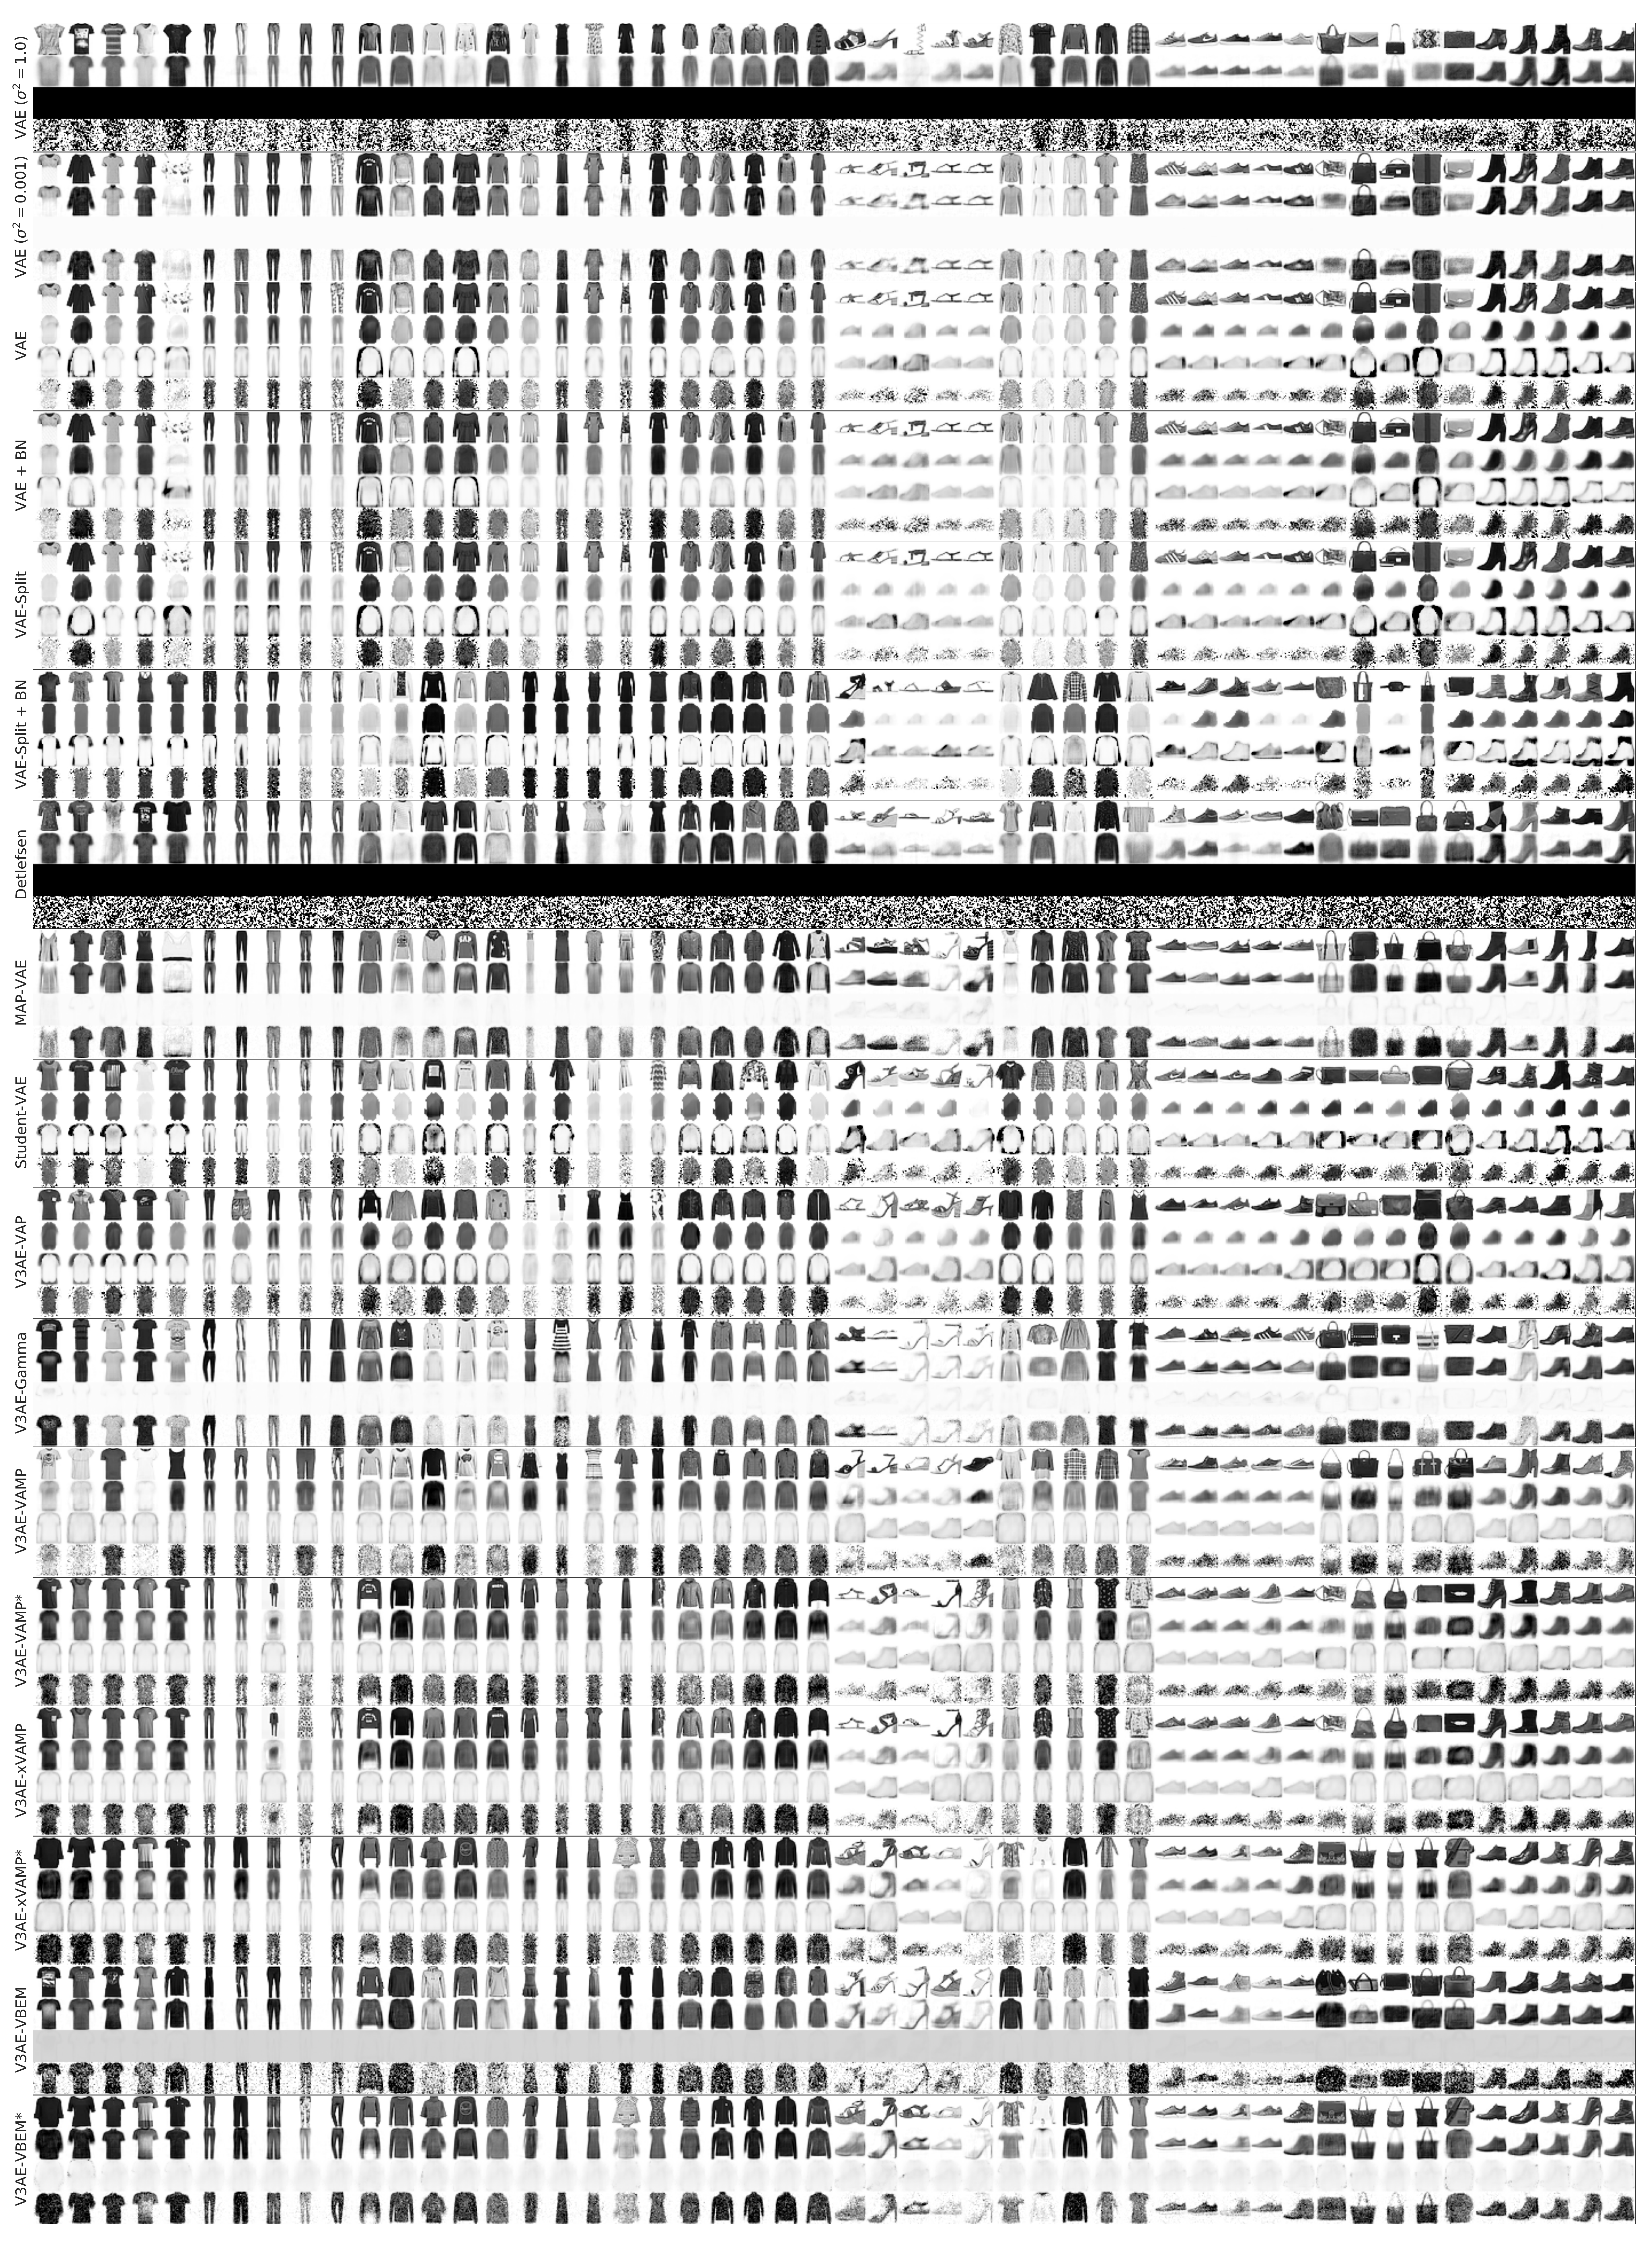}
    \caption{\captionVAE{Fashion MNIST}}
    \label{fig:fashion}
\end{figure}

\clearpage
\begin{figure}
    \centering
    \includegraphics[height=0.9\textheight]{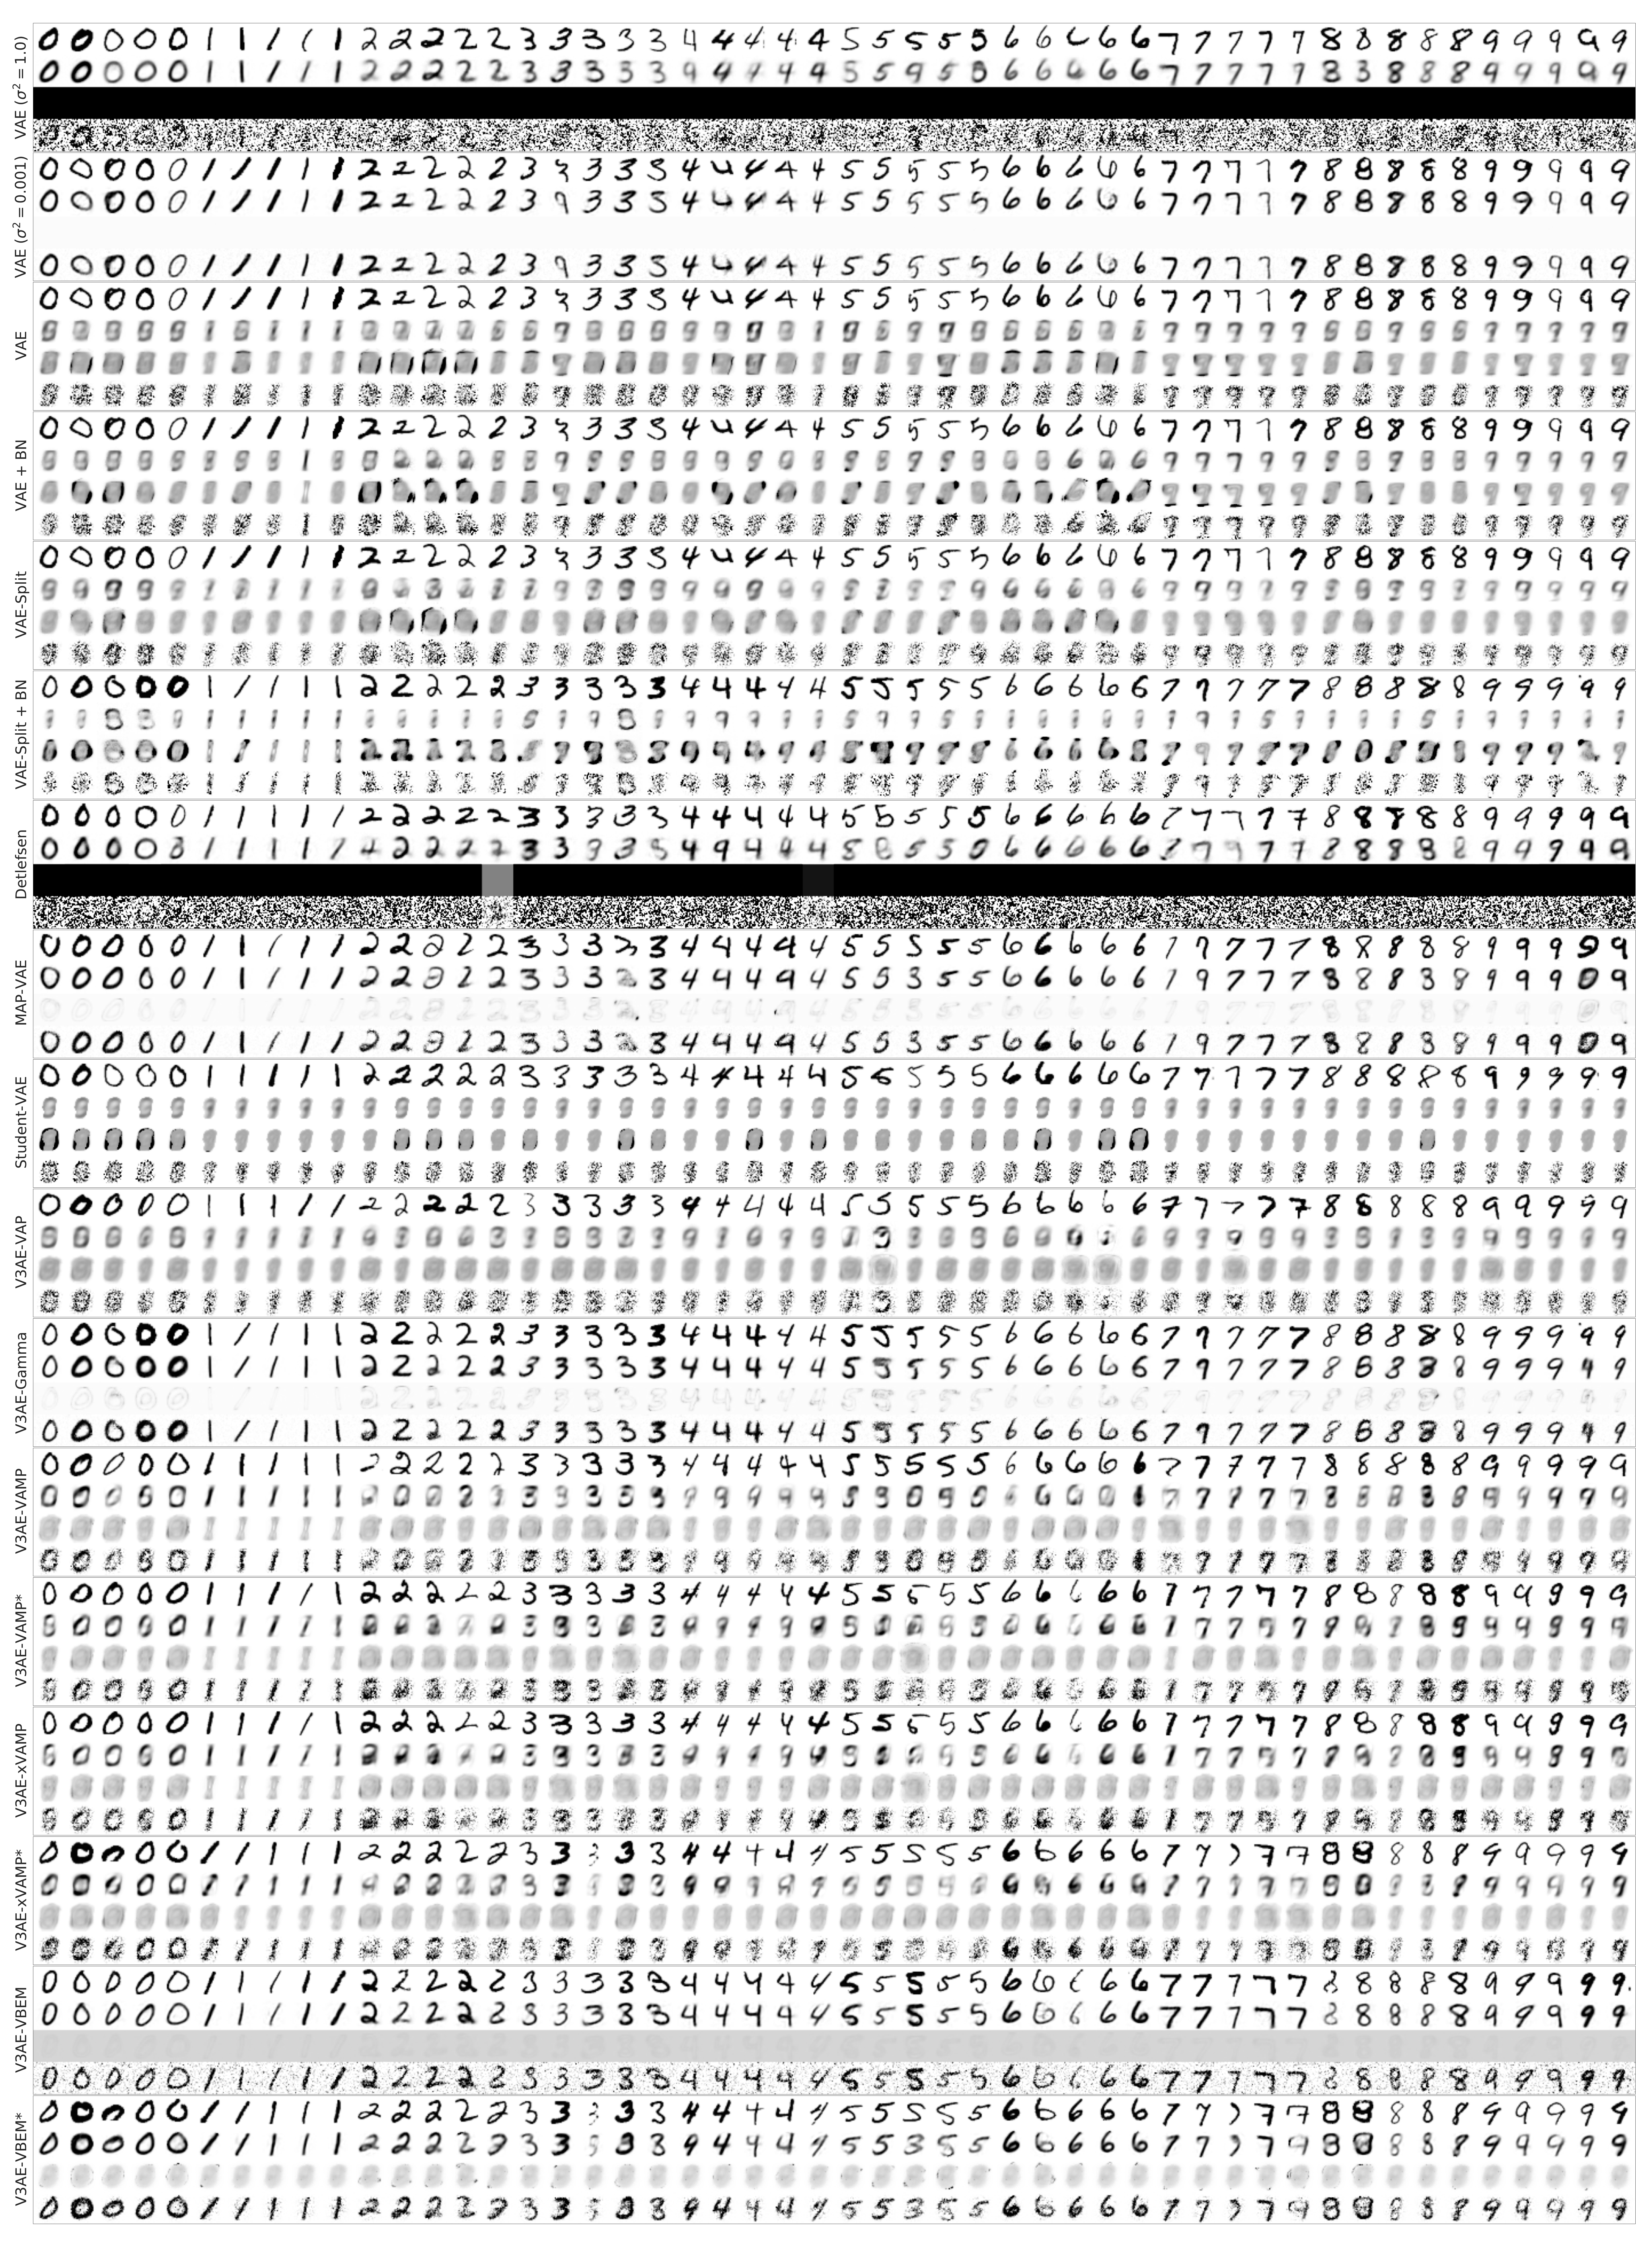}
    \caption{\captionVAE{MNIST}}
    \label{fig:mnist}
\end{figure}
